# Supplementary material for: Ensembling over Classifiers: a Bias-Variance Perspective
Source: arXiv:2206.10566 source file (2022-06-21)
Supplement: Supplementary file 1 [file appendix-results.tex]

\section{Estimating the bias and variance}
\label{app:experimental}
\begin{algorithm}[H]
    \caption{Conditional bias-variance estimates for ensembles of classification models}
    \label{alg:estimate-variance}
    \begin{algorithmic}
        \State {\bfseries Input:} ensemble size $k$, models $p\ens1, \ldots, p\ens n$, input $x$, label $y \in \{0, 1\}^c$, number of draws $N$ 
        \State $E \leftarrow 0$  \Comment{Total loss}
        \State $V_1, \ldots, V_c \leftarrow 0$ \Comment{Variance for class-$i$ predictions}
        \For{$i=1$ {\bfseries to} $N$}
            \State Draw $p\ens{i_1}, \ldots, p\ens{i_k}$ uniformly at random from $p\ens 1, \ldots, p\ens n$.
            \State $\tilde p \leftarrow \frac 1k \sum_{\ell=1}^k p\ens{i_\ell}(x)$ \Comment{Ensemble prediction}
            \State $E \leftarrow E + CE(y \mid \tilde p)$
            \For{$j=1$ {\bfseries to} $c$}
                \State $V_j \leftarrow V_j + \log \tilde p_j$
            \EndFor
        \EndFor
    \State $V \leftarrow - \log\left(\sum_{j=1}^c e^{\frac 1N V_j}\right)$
    \State $B \leftarrow \frac 1N E - V$
    \State {\bfseries return} Bias $B$, variance $V$.
    \end{algorithmic}
    \label{alg:bo}
\end{algorithm}

\begin{algorithm}[H]
    \caption{Bias-Variance}
    \label{alg:bias-variance}
    \begin{algorithmic}
        \State {\bfseries Input:} $(\{p^i\}_{i=1}^N, y \in \{0, 1\}^c)$
        \State $E \leftarrow 0$  \Comment{Total loss}
        \State $V_1, \ldots, V_c \leftarrow 0$ \Comment{Variance for class-$i$ predictions}
        \For{$i=1$ {\bfseries to} $N$}
            \State $E \leftarrow E + CE(y \mid  p^i)$
            \For{$j=1$ {\bfseries to} $c$}
                \State $V_j \leftarrow V_j + \log  p^i_j$
            \EndFor
        \EndFor
    \State $V \leftarrow - \log\left(\sum_{j=1}^c e^{\frac 1N V_j}\right)$
    \State $B \leftarrow \frac 1N E - V$
    \State {\bfseries return} Bias $B$, variance $V$.
    \end{algorithmic}
    \label{alg:bias-variance}
\end{algorithm}

\begin{algorithm}[H]
    \caption{Bootstrap samples}
    \label{alg:bootstrap}
    \begin{algorithmic}
        \State {\bfseries Input:} (x, y)
        \State $N \leftarrow length(x)$
         \State $\tilde{x} \leftarrow [], \tilde{y} \leftarrow []$
        \For{$i=1$ {\bfseries to} $N$}
            \State $j \leftarrow$ Uniform random number in $[1,N]$.
                \State Add $x[j]$ to $\tilde{x}$ and $y[j]$ to $\tilde{y}$. 
        \EndFor
    \State {\bfseries return} $\tilde{x}, \tilde{y}$.
    \end{algorithmic}
    \label{alg:bootstrap}
\end{algorithm}

\begin{algorithm}[H]
    \caption{Bootstrap bias-variance estimates for ensembles of classification models}
    \label{alg:estimate-variance}
    \begin{algorithmic}
        \State {\bfseries Input:} ensemble size $k$, input $x$, label $y \in \{0, 1\}^c$, number of bootstrap samples $N$ 
        \For{$i=1$ {\bfseries to} $N$}
            \State $x^{i}, y^{i} \leftarrow$ Bootstrap($x,y$)
                \State Train $k$ independent models on $(x^{i}, y^{i})$ named $p\ens{i_1}, \ldots, p\ens{i_k}$.
                \State $\tilde p^{i} \leftarrow \frac 1k \sum_{\ell=1}^k p\ens{i_\ell}(x)$ \Comment{Ensemble prediction}
            \For{$j=1$ {\bfseries to} $N$}
                \State $x^{ij}, y^{ij} \leftarrow$ Bootstrap($x^i,y^i$)
                \State Train $k$ independent models on $(x^{ij}, y^{ij})$ named $p\ens{ij_1}, \ldots, p\ens{ij_k}$.
                \State $\tilde p^{ij} \leftarrow \frac 1k \sum_{\ell=1}^k p\ens{ij_\ell}(x)$ \Comment{Ensemble prediction}
            \EndFor
            \State $B^{2i}, V^{2i} = BV(\{\tilde{p}^{ij}\}_{j=1}^N)$ 
        \EndFor
         \State $B^{2}, V^{2} = \frac{1}{N}\sum_{i=1}^N B^{2i}, \frac{1}{N}\sum_{i=1}^N V^{2i}$ \Comment{Bootstrap bias-variance estimates at level 2}
        \State $B^{1}, V^{1} = BV(\{\tilde{p}^{i}\}_{i=1}^N)$ \Comment{Bootstrap bias-variance estimates at level 1}
    \State $V \leftarrow \frac{V^1*V^1}{V^2}$ \Comment{Bootstrap variance estimate}
    \State $B \leftarrow \frac{B^1*B^1}{B^2}$ \Comment{Bootstrap bias estimate}
    \State {\bfseries return} Bias $B$, variance $V$.
    \end{algorithmic}
    \label{alg:bootstrap_bv}
\end{algorithm}
\section{Other Experimental Results}

\subsection{Multiple Depths}

\textbf{CIFAR 10 Corrupted test set}

\begin{figure*}[H]
\begin{subfigure}{.24\textwidth}
  \centering
  \includegraphics[scale=0.25]{figures/depths/cifar10/gn2/error.png}
  \caption{Cross entropy loss}
\end{subfigure}
\begin{subfigure}{.24\textwidth}
  \centering
  \includegraphics[scale=0.25]{figures/depths/cifar10/gn2/bias.png}
  \caption{Bias}
\end{subfigure}
\begin{subfigure}{.24\textwidth}
  \centering
\includegraphics[scale=0.25]{figures/depths/cifar10/gn2/variance.png}
  \caption{Variance}
\end{subfigure}
\begin{subfigure}{.24\textwidth}
  \centering
\includegraphics[scale=0.25]{figures/depths/cifar10/gn2/accuracy.png}
  \caption{Accuracy}
\end{subfigure}
\caption{Plots for bias, variance, error and accuracy with increasing ensemble size for CIFAR-10 corrupted dataset (gaussian noise with severity 2) when multiple networks are trained with different initial random seeds and different depths and then ensembled together in probability space. The line with depth=k denotes the setting where different models with depth=k are ensembled together. The line with depth-multiple denotes the setting where we first randomly sample a depth from [2,4,6] and then randomly sample a model from that. }
\end{figure*}

\textbf{CIFAR 100 corrupted}
\begin{figure}[H]
\begin{subfigure}{.24\textwidth}
  \centering
\includegraphics[scale=0.25]{figures/depths/cifar100/gn2/error.png}
  \caption{Cross entropy loss}
\end{subfigure}
\begin{subfigure}{.24\textwidth}
  \centering
\includegraphics[scale=0.25]{figures/depths/cifar100/gn2/bias.png}
  \caption{Bias}
\end{subfigure}
\begin{subfigure}{.24\textwidth}
  \centering
\includegraphics[scale=0.25]{figures/depths/cifar100/gn2/variance.png}
  \caption{Variance}
\end{subfigure}
\begin{subfigure}{.24\textwidth}
  \centering
\includegraphics[scale=0.25]{figures/depths/cifar100/gn2/accuracy.png}
  \caption{Accuracy}
\end{subfigure}
\caption{Plots for bias, variance, error and accuracy with increasing ensemble size for CIFAR-100 corrupted dataset (gaussian noise with severity 2) when multiple networks are trained with different initial random seeds and different depths and then ensembled together in probability space. The line with depth=k denotes the setting where different models with depth=k are ensembled together. The line with depth-multiple denotes the setting where we first randomly sample a depth from [4,6,8] and then randomly sample a model from that. }
\end{figure}

\subsection{Multiple Widths}

\textbf{CIFAR 10 - corrupted}
\begin{figure*}[H]
\begin{subfigure}{.24\textwidth}
  \centering
  \includegraphics[scale=0.25]{figures/widths/cifar10/gn2/error.png}
  \caption{Cross entropy loss}
\end{subfigure}
\begin{subfigure}{.24\textwidth}
  \centering
\includegraphics[scale=0.24]{figures/widths/cifar10/gn2/bias.png}
  \caption{Bias}
\end{subfigure}
\begin{subfigure}{.24\textwidth}
  \centering
\includegraphics[scale=0.25]{figures/widths/cifar10/gn2/variance.png}
  \caption{Variance}
\end{subfigure}
\begin{subfigure}{.24\textwidth}
  \centering
\includegraphics[scale=0.25]{figures/widths/cifar10/gn2/accuracy.png}
  \caption{Accuracy}
\end{subfigure}
\caption{Plots for bias, variance, error and accuracy with increasing ensemble size for CIFAR-10 corrupted dataset (gaussian noise with severity 2) when multiple networks are trained with different initial random seeds and different widths and then ensembled together in probability space. The line with width=k denotes the setting where different models with width=k are ensembled together. The line with depth-multiple denotes the setting where we first randomly sample a width from [10,20,30] and then randomly sample a model from that. }
\end{figure*}
%\newpage
%
\textbf{CIFAR 100 - corrupted}
\begin{figure*}[H]
\begin{subfigure}{.24\textwidth}
  \centering
  \includegraphics[scale=0.25]{figures/widths/cifar100/gn2/error.png}
  \caption{Cross entropy loss}
\end{subfigure}
\begin{subfigure}{.24\textwidth}
  \centering
\includegraphics[scale=0.25]{figures/widths/cifar100/gn2/bias.png}
  \caption{Bias}
\end{subfigure}
\begin{subfigure}{.24\textwidth}
  \centering
\includegraphics[scale=0.25]{figures/widths/cifar100/gn2/variance.png}
  \caption{Variance}
\end{subfigure}
\begin{subfigure}{.24\textwidth}
  \centering
\includegraphics[scale=0.25]{figures/widths/cifar100/gn2/accuracy.png}
  \caption{Accuracy}
\end{subfigure}
\caption{Plots for bias, variance, error and accuracy with increasing ensemble size for CIFAR-100 corrupted dataset (gaussian noise with severity 2) when multiple networks are trained with different initial random seeds and different widths and then ensembled together in probability space. The line with width=k denotes the setting where different models with width=k are ensembled together. The line with depth-multiple denotes the setting where we first randomly sample a width from [10, 20, 30] and then randomly sample a model from that. }
\end{figure*}
